# Supplementary material for: Opposite impact of thermal expansion and phonon anharmonicity on the phonon-limited resistivity of elemental metals from first principles
Source: arXiv:2511.17478 ancillary file (2026-02-03)
Supplement: Supplementary file 1 [file supp.pdf]

# Supplemental Information to
# Antagonistic impact of thermal expansion and phonon anharmonicity on the phonon-limited resistivity of elemental metals from first principles

Ao Wang,[1] Junwen Yin,[2,1] Félix Antoine Goudreault,[3] Michel Côté,[3] Olle Hellman,[4] and Samuel Poncé[1,5,*]

[1] *European Theoretical Spectroscopy Facility, Institute of Condensed Matter and Nanosciences, Université catholique de Louvain, Chemin des Étoiles 8, B-1348 Louvain-la-Neuve, Belgium.*
[2] *Scientific Computing Department, Science and Technology Facilities Council, UK Research and Innovation, Daresbury Laboratory, Keckwick Lane, Daresbury, WA4 4AD, UK.*
[3] *Département de Physique et Institut Courtois, Université de Montréal, C. P. 6128, Succursale Centre-Ville, Montréal, Québec, H3C 3J7, Canada.*
[4] *Department of Molecular Chemistry and Materials Science, Weizmann Institute of Science, Rehovoth 76100, Israel.*
[5] *WEL Research Institute, Avenue Pasteur 6, 1300 Wavre, Belgium.*

(Dated: November 21, 2025)

## S1. COMPUTATIONAL DETAILS FOR THE ANHARMONIC CALCULATIONS IN LEAD

The first-principles calculations for Pb done with the Quantum ESPRESSO (QE) package [1, 2] with the same fully-relativistic ultrasoft pseudopotential (USPP) [3] with local-density approximation (LDA) [4] from the PSLibrary version 0.2.2 [5], as in Ref. [6] was used the calculation. Spin-orbit coupling (SOC) is included. We use a plane wave truncation of 90 Ry with a Gaussian smearing of 1 mRy with a shifted $36 \times 36 \times 36$ Monkhorst-Pack grid [7, 8]. The phonon without anharmonic effect are calculated with the density-functional perturbation theory (DFPT) [9, 10]. An $8 \times 8 \times 8$ **q**-mesh with a threshold for the self-consistent Sternheimer equation of $10^{-16}$ Ry is used. We use the same thermal expansion as Ref. [6, 11] with the lattice parameters 4.882, 4.887, 4.900, 4.916, 4.935, 4.955, 4.977, 5.000 Å, corresponding to the temperatures 10, 110, 210, 310, 410, 510, and 610 K, respectively. For the stochastic TDEP (sTDEP) [12, 13] calculations, a $6 \times 6 \times 6$ supercell is used. For each temperature, six iterations are needed to converge the phonon dispersions where the number of configurations used in step $l$ is $2^{(l-1)}$, which gives 63 configurations in total. We present in Fig. S1 the convergence with iteration number of the phonon dispersion at 210, 410, and 610 K when anharmonic effect are included and in Fig. S2 when both anharmonic and thermal expansion effects are included.

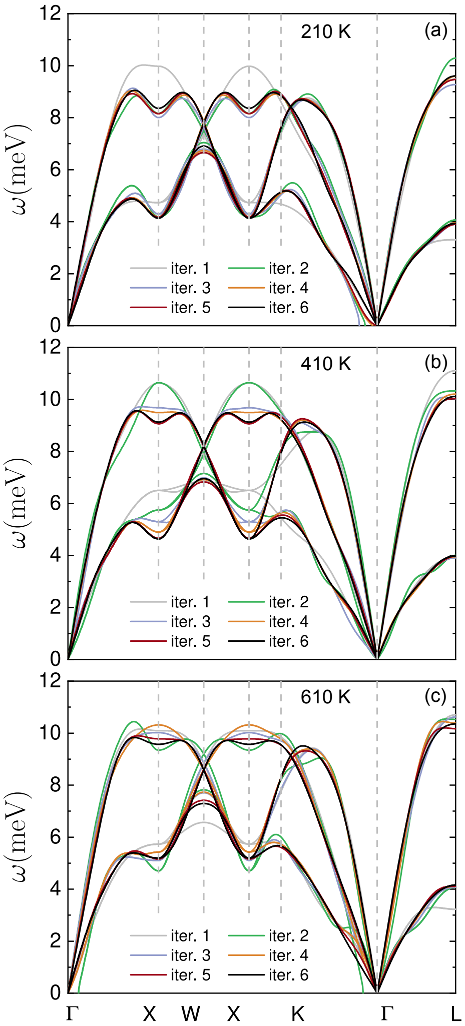


FIG. S1. Phonon dispersion of Pb with phonon anharmonicity at (a) 210 K, (b) 410 K, and (c) 610 K with respect to the number of iterations.

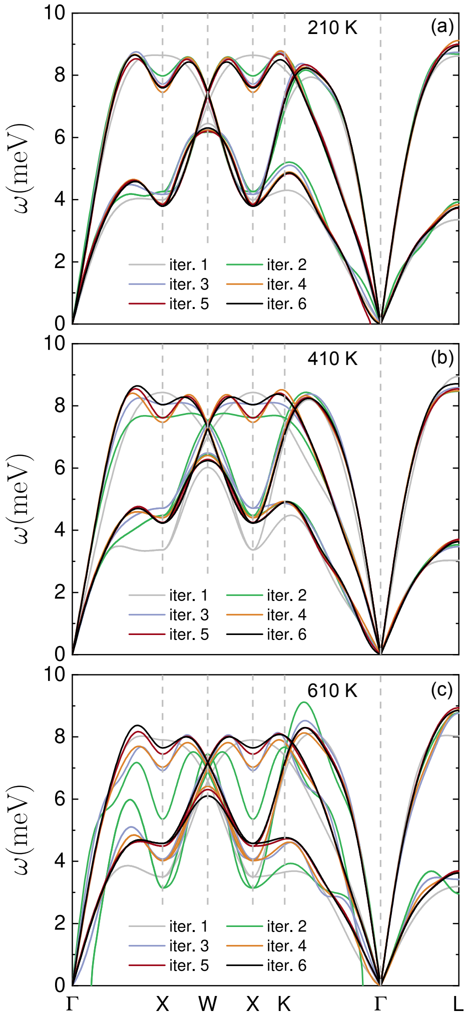


FIG. S2. Phonon dispersion of Pb with thermal expansion and anharmonicity at (a) 210 K, (b) 410 K, and (c) 610 K with respect to the number of iterations.

## S2. COMPUTATIONAL DETAILS FOR THE RESISTIVITY CALCULATIONS IN LEAD

We interpolate the Hamiltonian, dynamical matrices and electron-phonon matrix elements using EPW from a coarse $16 \times 16 \times 16$ **k**-point and $8 \times 8 \times 8$ **q** grids to a dense $60 \times 60 \times 60$ **k** and **q** grids. We use an adaptive smearing approach [14] for the energy-conserving delta functions when solving the Boltzmann transport equation. We confirm in Fig. S3 that we recover the computed electrical resistivity without thermal expansion and phonon anharmonicity from Ref. 6. We also show in Fig. S4(a) the impact of thermal expansion on the electronic band structure and the Fermi surface of Pb without thermal expansion in Fig. S4(b).

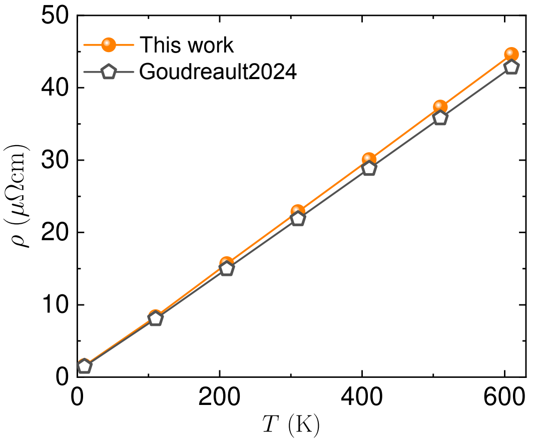


FIG. S3. Electrical resistivity of Pb with spin-orbit-coupling from 10 to 610 K calculated by the iterative BTE without thermal expansion and phonon anharmonicity. Gray pentagon are results from Ref. [6].

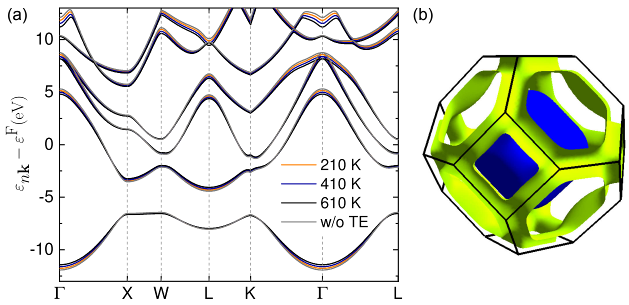


FIG. S4. (a) Electron band structure of Pb including thermal expansion (TE) effect at 210, 410, and 610 K compared to the case without TE. The energies are presented with respect to the Fermi level $\varepsilon^{\mathrm{F}}$. (b) The Fermi surface of Pb without TE.

## S3. COMPUTATIONAL DETAILS FOR THE ANHARMONIC AND RESISTIVITY CALCULATIONS IN ALUMINUM AND NIOBIUM

For the calculations of Al and Nb, we use PBE [15] scalar relativistic optimized norm-conserving Vanderbilt pseudopotential (ONCV) [16] from PseudoDojo [17]. Due to their lower atomic number than Pb, we neglected SOC. We use a plane wave truncation of 40 Ry with a Marzari-Vanderbilt-DeVita-Payne cold smearing [18] of 15 mRy with a 46 × 46 × 46 Monkhorst-Pack grid [7, 8] for Al. As for the calculation of Nb, a plane wave truncation of 65 Ry with a Gaussian smearing of 15 mRy with a 28 × 28 × 28 Monkhorst-Pack grid [7, 8] is used. A 6 × 6 × 6 **q**-mesh with a threshold for the self-consistent Sternheimer equation of $10^{-12}$ Ry and $10^{-16}$ Ry are applied to Al and Nb to obtain the phonon properties. The temperature-dependent lattice parameters for Al and Nb are extracted from previous experiments, with 4.0680, 4.0909, and 4.1197 Å at 481, 682, and 900 K for Al [19], and 3.319, 3.334, and 3.350 Å at 1000, 1500, and 2000 K for Nb [20]. The lattice parameter without TE is also extracted from previous experiments, as 4.0315 Å for Al [21] and 3.295 Å for Nb [20]. We show the calculated phonon dispersions of Al at 481, 682, and 900 K with TDEP with respect to iteration steps with thermal expansion in Fig. S5. With five iteration steps, the phonon dispersion is converged for the three investigated temperatures. The phonon dispersion of Al including lattice thermal expansion and including both thermal expansion and the phonon anharmonicity is shown in Fig. S6.

Similarly, for Nb, we show the phonon dispersions at 1000, 1500, and 2000 K with TDEP with respect to iteration steps with thermal expansion in Fig. S7. With four iteration steps, the phonon dispersion is converged for the three investigated temperatures. Phonon dispersions including lattice thermal expansion and including both thermal expansion and the phonon anharmonicity is reported in Fig. S8. To verify the reliability of our calculated resistivity, we further show the comparison of the band structure of Pb, Al, and Nb obtained by EPW interpolation and DFT in Fig. S9. The EPW interpolated bands reproduce perfectly the electronic band structure. We also show the convergence for the IBTE calculations in Al and Nb with respect to the fine **k** and **q**-grids in Fig. S10. For the electrical resistivity of Al, we focus on the results from 481 to 900 K, and the data calculated with the three grids are nearly the same, as shown in Fig. S10(a). For the electrical resistivity of Nb from 0 to 3000 K, the data obtained with the three meshes are nearly the same. Therefore, in our calculation of the resistivity with TE and with both TE and anharmonicity, a 50 × 50 × 50 **k** and **q**-grid is used for the IBTE calculation for both Al and Nb to ensure convergence.

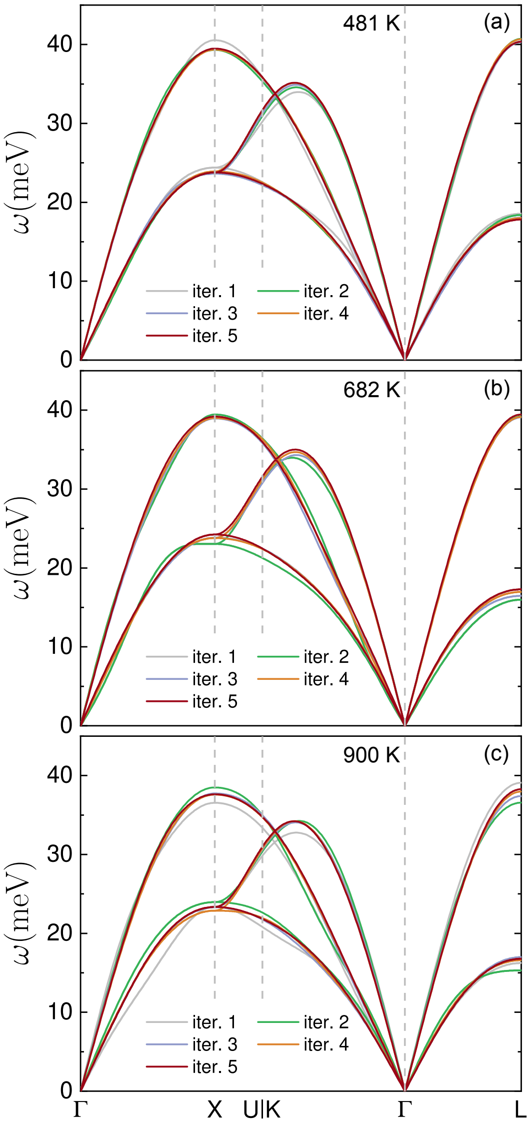


FIG. S5. Phonon dispersion of Al with thermal expansion and phonon anharmonicity at (a) 481 K, (b) 682 K, and (c) 900 K with respect to the iteration steps.

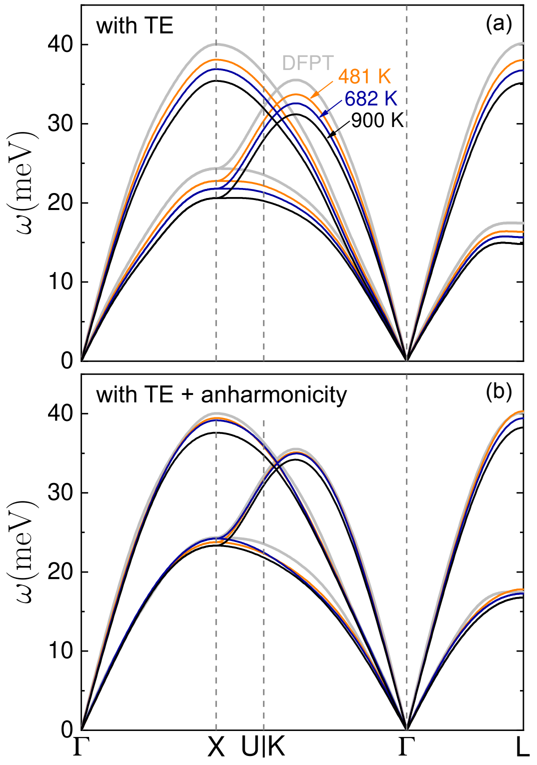


FIG. S6. Phonon dispersion of Al including (a) lattice thermal expansion (TE) effect (b) with TE and phonon anharmonicity. In all cases the gray line is the harmonic phonon dispersion computed with density functional perturbation theory (DFPT) without TE.

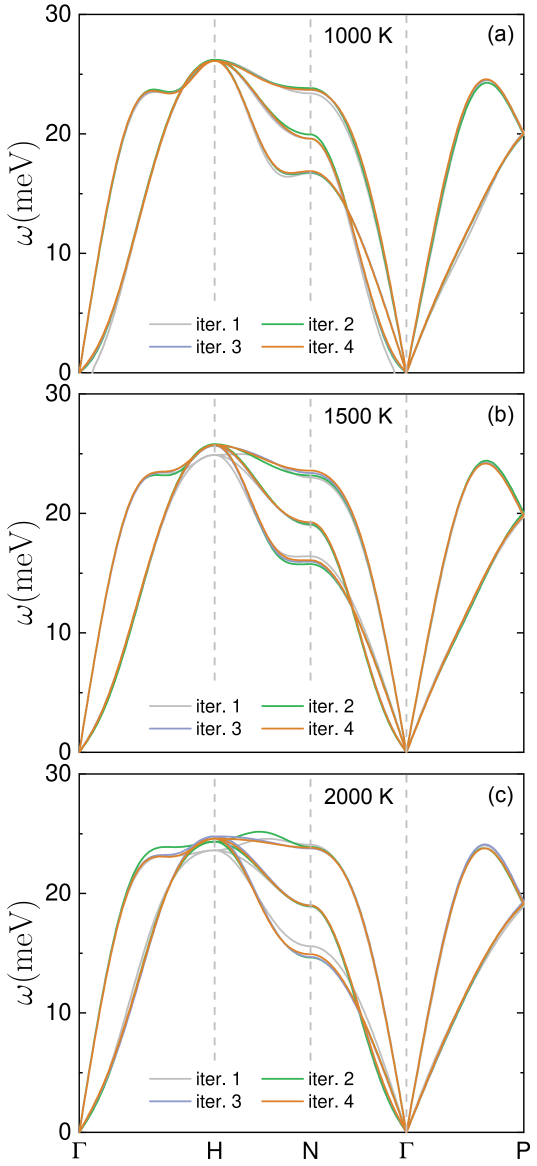


FIG. S7. Phonon dispersion of Nb with thermal expansion and phonon anharmonicity at (a) 1000 K, (b) 1500 K, and (c) 2000 K with respect to the number of iterations.

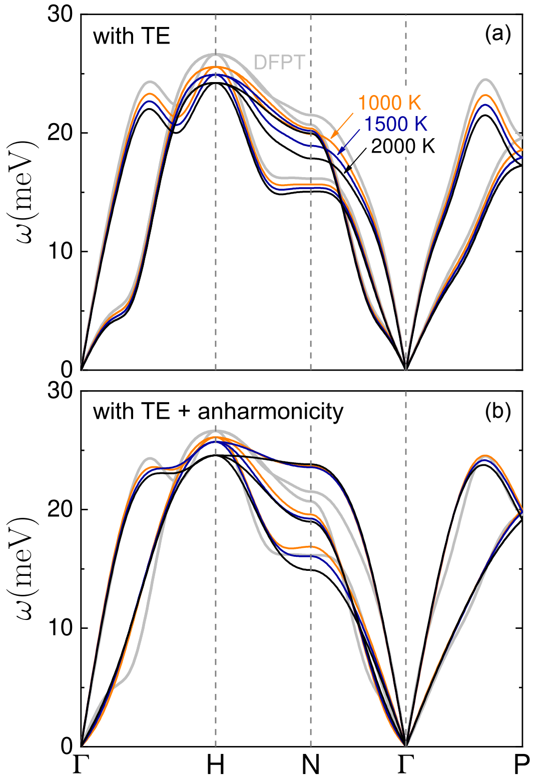


FIG. S8. Phonon dispersion of Nb including (a) lattice thermal expansion (TE) effect (b) with TE and phonon anharmonicity. In all cases the gray line is the harmonic phonon dispersion with density functional perturbation theory (DFPT) without TE.

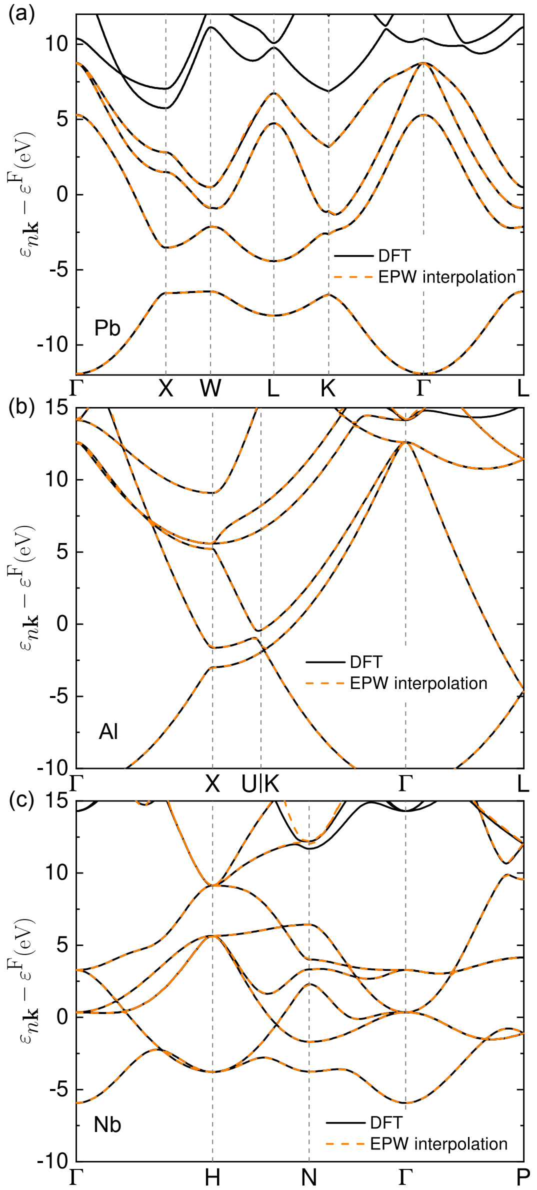


FIG. S9. EPW interpolation and DFT electronic band structure of (a) Pb, (b) Al, and (c) Nb. The energies are presented with respect to the Fermi level $\varepsilon^{\mathrm{F}}$.

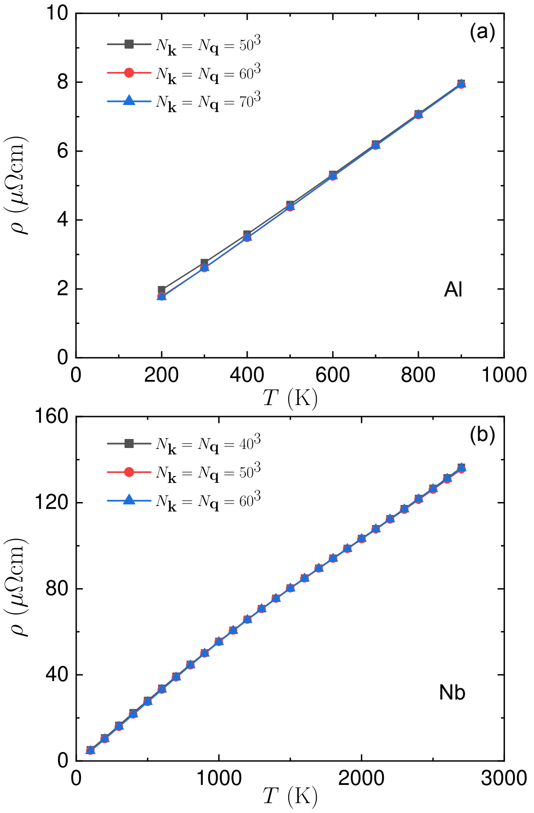


FIG. S10. Convergence study with respect to the fine $\mathbf{k}$ and $\mathbf{q}$ grids for the resistivity of (a) Al and (b) Nb.

* samuel.ponce@uclouvain.be


[1] P. Giannozzi, O. Andreussi, T. Brumme, O. Bunau, M. Buongiorno Nardelli, M. Calandra, R. Car, C. Cavazzoni, D. Ceresoli, M. Cococcioni, N. Colonna, I. Carnimeo, A. Dal Corso, S. de Gironcoli, P. Delugas, R. A. DiStasio, A. Ferretti, A. Floris, G. Fratesi, G. Fugallo, R. Gebauer, U. Gerstmann, F. Giustino, T. Gorni, J. Jia, M. Kawamura, H.-Y. Ko, A. Kokalj, E. Küçükbenli, M. Lazzeri, M. Marsili, N. Marzari, F. Mauri, N. L. Nguyen, H.-V. Nguyen, A. Otero-de-la Roza, L. Paulatto, S. Poncé, D. Rocca, R. Sabatini, B. Santra, M. Schlipf, A. P. Seitsonen, A. Smogunov, I. Timrov, T. Thonhauser, P. Umari, N. Vast, X. Wu, and S. Baroni, Advanced capabilities for materials modelling with quantum espresso, Journal of Physics: Condensed Matter **29**, 465901 (2017).

[2] P. Giannozzi, O. Baseggio, P. Bonfà, D. Brunato, R. Car, I. Carnimeo, C. Cavazzoni, S. de Gironcoli, P. Delugas, F. Ferrari Ruffino, A. Ferretti, N. Marzari, I. Timrov, A. Urru, and S. Baroni, Quantum espresso toward the exascale, The Journal of Chemical Physics **152**, 154105 (2020).

[3] D. Vanderbilt, Soft self-consistent pseudopotentials in a generalized eigenvalue formalism, Physical Review B **41**, 7892–7895 (1990).

[4] J. P. Perdew and A. Zunger, Self-interaction correction to density-functional approximations for many-electron systems, Physical Review B **23**, 5048–5079 (1981).

[5] A. Dal Corso, Pseudopotentials periodic table: From H to Pu, Computational Materials Science **95**, 337–350 (2014).

[6] F. A. Goudreault, S. Poncé, F. Giustino, and M. Côté, Effects of spin-orbit coupling and thermal expansion on the phonon-limited resistivity of pb from first principles (2024), arXiv:2410.20157.

[7] H. J. Monkhorst and J. D. Pack, Special points for brillouin-zone integrations, Physical Review B **13**, 5188–5192 (1976).

[8] J. D. Pack and H. J. Monkhorst, "special points for brillouin-zone integrations"—a reply, Physical Review B **16**, 1748–1749 (1977).

[9] S. Baroni, P. Giannozzi, and A. Testa, Green's-function approach to linear response in solids, Physical Review Letters **58**, 1861–1864 (1987).

[10] X. Gonze and J.-P. Vigneron, Density-functional approach to nonlinear-response coefficients of solids, Physical Review B **39**, 13120–13128 (1989).

[11] R. Feder and A. S. Nowick, Use of thermal expansion measurements to detect lattice vacancies near the melting point of pure lead and aluminum, Physical Review **109**, 1959–1963 (1958).

[12] F. Knoop, N. Shulumba, A. Castellano, J. P. A. Batista, R. Farris, M. J. Verstraete, M. Heine, D. Broido, D. S. Kim, J. Klarbring, I. A. Abrikosov, S. I. Simak, and O. Hellman, TDEP: Temperature dependent effective potentials, Journal of Open Source Software **9**, 6150 (2024).

[13] N. Shulumba, O. Hellman, and A. J. Minnich, Lattice thermal conductivity of polyethylene molecular crystals from first-principles including nuclear quantum effects, Physical Review Letters **119**, 185901 (2017).

[14] F. Macheda and N. Bonini, Magnetotransport phenomena in *p*-doped diamond from first principles, Physical Review B **98**, 201201(R) (2018).

[15] J. P. Perdew, K. Burke, and M. Ernzerhof, Generalized gradient approximation made simple, Physical Review Letters **77**, 3865–3868 (1996).

[16] D. R. Hamann, Optimized norm-conserving vanderbilt pseudopotentials, Physical Review B **88**, 085117 (2013).

[17] M. van Setten, M. Giantomassi, E. Bousquet, M. Verstraete, D. Hamann, X. Gonze, and G.-M. Rignanese, The pseudodojo: Training and grading a 85 element optimized norm-conserving pseudopotential table, Computer Physics Communications **226**, 39–54 (2018).

[18] N. Marzari, D. Vanderbilt, A. De Vita, and M. C. Payne, Thermal contraction and disordering of the al(110) surface, Physical Review Letters **82**, 3296–3299 (1999).

[19] S. Nenno and J. W. Kauffman, Detection and determination of equilibrium vacancy concentrations in aluminum, Journal of the Physical Society of Japan **15**, 220–226 (1960).

[20] K. Wang and R. R. Reeber, The role of defects on thermophysical properties: Thermal expansion of V, Nb, Ta, Mo and W, Materials Science and Engineering: R: Reports **23**, 101–137 (1998).

[21] J. Bandyopadhyay and K. Gupta, Low temperature lattice parameters of Al and Al-Zn alloys and grüneisen parameter of Al, Cryogenics **18**, 54–55 (1978).
